# Supplementary material for: Chemistry Lab Automation via Constrained Task and Motion Planning
Source: arXiv:2212.09672 source file (2023-03-27)
Supplement: Supplementary file 1 [file appendix.tex]

\subsection{Object Position Estimation Error Due to Hand-Eye Calibration Error}
\label{app:perception-error}
\begin{remark} 
The object position estimation error L2 norm $\| \delta ^{\mathcal{I}}\bm{p}_{\mathcal{O}}\| = \| ^{\mathcal{I}}\tilde{\bm{p}}_{\mathcal{O}} - ^{\mathcal{I}}\bm{p}_{\mathcal{O}} \|$ caused by the hand-eye calibration error decreases as the camera capturing the object pose is closer to the object, i.e., lower $ \| ^{\mathcal{C}}\bm{p}_{\mathcal{O}}  \|$.
\end{remark}

${\mathcal{I}}$ is the inertial or the world frame, ${\mathcal{C}}$ is the camera frame, and ${\mathcal{T}}$ is the robot tool or end-effector frame.
% We assume that the errors of the robot object pose estimation in the camera frame and the robot tool pose estimation using the robot encoders are negligible in front of the hand-eye calibration error.
We assume that the errors of object pose estimation in the camera frame and the robot tool pose estimation using the robot encoders are negligible compared to the hand-eye calibration error.
We can write down:
\begin{equation}
\begin{array}{l}
^{\mathcal{I}}\tilde{\bm{T}}_{\mathcal{O}} = ~^{\mathcal{I}}\tilde{\bm{T}}_{\mathcal{T}}~ ^{\mathcal{T}}\tilde{\bm{T}}_{\mathcal{C}}~ ^{\mathcal{C}}\tilde{\bm{T}}_{\mathcal{O}}
 = \begin{pmatrix}
  ^{\mathcal{I}}\bm{R}_{\mathcal{O}} & ^{\mathcal{I}}{\bm{p}}_{\mathcal{O}} \\
  \bm{0} & 1 
 \end{pmatrix} = 
 \\ 
 \begin{pmatrix}
  ^{\mathcal{I}}\bm{R}_{\mathcal{T}} & ^{\mathcal{I}}{\bm{p}}_{\mathcal{T}} \\
  \bm{0} & 1 
 \end{pmatrix} 
  \begin{pmatrix}
  ^{\mathcal{T}}\bm{R}_{\mathcal{C}} ~ \bm{R}_{\epsilon} & ^{\mathcal{T}}{\bm{p}}_{\mathcal{C}} + \bm{p}_{\epsilon}\\
  \bm{0} & 1 
 \end{pmatrix}
\begin{pmatrix}
  ^{\mathcal{C}}\bm{R}_{\mathcal{O}} & ^{\mathcal{C}}{\bm{p}}_{\mathcal{O}} \\
  \bm{0} & 1 
\end{pmatrix},
\end{array}
\end{equation}
where $\bm{R}_{\epsilon}$ and $\bm{p}_{\epsilon}$ results from the camera calibration error. In the case of no error, $\bm{R}_{\epsilon} = \bm{I}$ and $\bm{p}_{\epsilon}=\bm{0}$. From this equation, we can compute $ \delta ^{\mathcal{I}}\bm{p}_{\mathcal{O}}$ as:
\begin{equation}
\begin{array}{l}
\delta ^{\mathcal{I}}\bm{p}_{\mathcal{O}} = ^{\mathcal{I}}\tilde{\bm{p}}_{\mathcal{O}} - ^{\mathcal{I}}\bm{p}_{\mathcal{O}} = \\
^{\mathcal{I}}\bm{R}_{\mathcal{T}} ~ ^{\mathcal{T}}\bm{R}_{\mathcal{C}} ~ ( \bm{R}_{\epsilon} - \bm{I}) ~ ^{\mathcal{C}}{\bm{p}}_{\mathcal{O}} + ^{\mathcal{I}}\bm{R}_{\mathcal{T}} ~ \bm{p}_{\epsilon}
\end{array}
\end{equation}
Using the triangle inequality for vectors and matrix norm submultiplicative lemmas, we can deduce:
\begin{equation}
\begin{array}{l}
\| \delta ^{\mathcal{I}}\bm{p}_{\mathcal{O}} \| = \| ^{\mathcal{I}}\bm{R}_{\mathcal{T}} ~ ^{\mathcal{T}}\bm{R}_{\mathcal{C}} ~ ( \bm{R}_{\epsilon} - \bm{I}) ~ ^{\mathcal{C}}{\bm{p}}_{\mathcal{O}} + ^{\mathcal{I}}\bm{R}_{\mathcal{T}} ~ \bm{p}_{\epsilon} \| \leq   \\ \|^{\mathcal{I}}\bm{R}_{\mathcal{T}}\| ~ \|^{\mathcal{T}}\bm{R}_{\mathcal{C}}\| ~ \|( \bm{R}_{\epsilon} - \bm{I})\| ~ \|^{\mathcal{C}}{\bm{p}}_{\mathcal{O}}\| + \|^{\mathcal{I}}\bm{R}_{\mathcal{T}}\| ~ \| \bm{p}_{\epsilon} \|
\\ \leq
\|\bm{R}_{\epsilon} - \bm{I}\| ~ \|^{\mathcal{C}}{\bm{p}}_{\mathcal{O}}\| +  \| \bm{p}_{\epsilon} \|.
\end{array}
\end{equation}
This equation proves that as the object-camera distance decreases when $\bm{R}_{\epsilon} \neq \bm{I}$ ,  the upper bound of the perception error (object position estimation) decreases.
